# Supplementary material for: Ab initio constraints on silica melting to 500 GPa
Source: arXiv:2307.05444 source file (2023-11-18)

# *Ab initio* constraints on silica melting to 500 GPa
# Supplemental Information

Ming Geng (耿明) [1] and Chris E. Mohn[1,2,*]
[1] *Centre for Earth Evolution and Dynamics (CEED) and Centre for Planetary Habitability (PHAB), University of Oslo, N-0315 Oslo, Norway* and
[2] *Department of Chemistry and Center for Materials Science and Nanotechnology, University of Oslo, Oslo 0371, Norway*
(Dated: November 17, 2023)

TABLE S1: Simulation temperature, average pressure, densities and waiting time, $\tau_{\text{equilibrium}}$, before freezing or melting in two-phase *ab initio* NVT MD runs. The first column "solid phase" refers to the crystal structure in the solid portion of the simulation box before the simulation is launched. Simulations with frozen-in defects in the solid state after the run has terminated is labeled as "defects" (i.e. a single Si is located at an interstitial site) or more "extended defects" (where several atoms have exchange positions compared to the ideal crystal structure). Typical error-bars in the equilibrium pressures are between 2 and 5 GPa.

| solid phase | T (K) | P (GPa) | $\rho$ (g/cm$^3$) | $\tau_{\text{equilibrium}}$ (ps) | final phase |
|---|---|---|---|---|---|
| stishovite | 5750 | 78 | 4.49 | 6.0 | L |
| stishovite | 5750 | 69 | 4.37 | 5.2 | L |
| stishovite | 5750 | 59 | 4.24 | 3.0 | L |
| stishovite | 5500 | 60 | 4.37 | 10.4 | L |
| stishovite | 5500 | 55 | 4.24 | 3.0 | L |
| stishovite | 5500 | 48 | 4.12 | 3.0 | L |
| stishovite | 5500 | 43 | 4.00 | 2.0 | L |
| stishovite | 5250 | 55 | 4.24 | 9.5 | L |
| stishovite | 5250 | 41 | 4.00 | 3.6 | L |
| stishovite | 5250 | 37 | 3.89 | 1.9 | L |
| stishovite | 5000 | 45 | 4.12 | 5.0 | L |
| stishovite | 5500 | 100 | 4.93 | 6.0 | S (stishovite w defects) |
| stishovite | 5500 | 85 | 4.77 | 8.8 | S (stishovite w extended defects) |
| stishovite | 5500 | 70 | 4.64 | 8.4 | S (stishovite) |
| stishovite | 5500 | 55 | 4.50 | 19.4 | S (stishovite) |
| stishovite | 5250 | 100 | 4.93 | 8.2 | S (stishovite) |
| stishovite | 5250 | 86 | 4.77 | 4.5 | S (stishovite) |
| stishovite | 5250 | 62 | 4.50 | 6.6 | S (stishovite) |
| stishovite | 5250 | 58 | 4.37 | 5.2 | S (stishovite) |
| $\beta$-stishovite | 6000 | 90 | 4.60 | 3.0 | L |
| $\beta$-stishovite | 6000 | 100 | 4.74 | 8.0 | L |
| $\beta$-stishovite | 6250 | 100 | 4.74 | 2.4 | L |
| $\beta$-stishovite | 6250 | 111 | 4.88 | 7.2 | L |
| $\beta$-stishovite | 6250 | 131 | 5.03 | 18.0 | L |
| $\beta$-stishovite | 6500 | 146 | 5.19 | 5.4 | L |
| $\beta$-stishovite | 5750 | 81 | 4.74 | 13.8 | S ($\beta$-stishovite) |
| $\beta$-stishovite | 5750 | 75 | 4.60 | 7.8 | S ($\beta$-stishovite |
| $\beta$-stishovite | 6250 | 141 | 5.12 | 8.0 | S ($\beta$-stishovite w. defect cluster) |
| $\beta$-stishovite | 6250 | 156 | 5.35 | 14.0 | S ($\beta$-stishovite) |
| $\beta$-stishovite | 6250 | 182 | 5.52 | 16.4 | S ($\beta$-stishovite) |
| $\beta$-stishovite | 6000 | 180 | 5.52 | 4.2 | S ($\beta$-stishovite) above stab. field |
| $\beta$-stishovite | 6000 | 158 | 5.35 | 8.0 | S ($\beta$-stishovite) |
| $\beta$-stishovite | 6000 | 136 | 5.19 | 4.0 | S ($\beta$-stishovite) |
| $\beta$-stishovite | 6000 | 117 | 5.03 | 5.6 | S ($\beta$-stishovite w. extended defects) |
| $\beta$-stishovite | 6000 | 102 | 4.88 | 5.1 | S ($\beta$-stishovite) |
| seifertite | 6500 | 214 | 5.77 | 22.0 | S (seifertite) |
| seifertite | 6500 | 141 | 5.28 | 11.4 | L |
| seifertite | 6750 | 161 | 5.28 | 8.4 | L |

* chrism@kjemi.uio.no

| | | | | | |
|---|---|---|---|---|---|
| seifertite | 6750 | 179 | 5.43 | 8.3 | L |
| seifertite | 7000 | 180 | 5.43 | 6.1 | L |
| seifertite | 7000 | 164 | 5.28 | 3.0 | L |
| pyrite | 6500 | 152 | 5.78 | 12.6 | S (pyrite) |
| pyrite | 6500 | 178 | 5.62 | 7.4 | S (pyrite) |
| pyrite | 6750 | 173 | 5.32 | 14.6 | S (pyrite) |
| pyrite | 6750 | 194 | 5.47 | 2.0 | S (pyrite) |
| pyrite | 6750 | 218 | 5.32 | 2.0 | S (pyrite) |
| pyrite | 6750 | 245 | 5.17 | 2.6 | S (pyrite) |
| pyrite | 7000 | 248 | 5.17 | 2.8 | S (pyrite) |
| pyrite | 7000 | 224 | 5.32 | 4.4 | S (pyrite) |
| pyrite | 7250 | 224 | 5.94 | 8.3 | S (pyrite) |
| pyrite | 7250 | 251 | 5.17 | 3.0 | S (pyrite) |
| pyrite | 7250 | 289 | 6.28 | 4.0 | S (pyrite) |
| pyrite | 7500 | 282 | 6.28 | 3.2 | S (pyrite) |
| pyrite seed 2 | 7500 | 284 | 6.28 | 5.2 | S (pyrite) |
| pyrite | 7500 | 314 | 6.47 | 2.3 | S (pyrite) |
| pyrite | 7750 | 319 | 4.88 | 4.5 | S (pyrite) |
| pyrite | 8000 | 330 | 6.47 | 11.9 | S (pyrite) |
| pyrite | 8000 | 357 | 6.66 | 11.1 | S (pyrite) |
| pyrite | 8000 | 399 | 6.85 | 4.2 | S (pyrite) |
| pyrite | 8000 | 441 | 7.06 | 13.9 | S (pyrite) |
| pyrite | 8250 | 400 | 6.85 | 2.6 | S (pyrite) |
| pyrite seed 2 | 8250 | 399 | 6.85 | 2.8 | S (pyrite) |
| pyrite | 8250 | 443 | 7.06 | 14.4 | S (pyrite) |
| pyrite seed 2 | 8250 | 443 | 7.06 | 5.0 | S (pyrite) |
| pyrite | 8500 | 546 | 4.21 | 9.6 | S (pyrite) |
| pyrite | 8500 | 494 | 4.34 | 32.5 | S (pyrite |
| pyrite | 7000 | 206 | 5.62 | 5.0 | L |
| pyrite | 7250 | 250 | 5.32 | 14.2 | L |
| pyrite | 7250 | 228 | 5.77 | 8.8 | L |
| pyrite | 7250 | 205 | 5.62 | 2.7 | L |
| pyrite | 7500 | 209 | 5.62 | 1.8 | L |
| pyrite | 7500 | 249 | 5.94 | 4.4 | L |
| pyrite | 7500 | 229 | 5.77 | 1.5 | L |
| pyrite | 7500 | 280 | 6.11 | 8.8 | L |
| pyrite | 7750 | 311 | 5.02 | 5.0 | L |
| pyrite | 7750 | 283 | 5.17 | 2.8 | L |
| pyrite | 7750 | 257 | 5.32 | 2.4 | L |
| pyrite | 8000 | 306 | 6.28 | 2.7 | L |
| pyrite | 8000 | 286 | 5.17 | 2.0 | L |
| pyrite | 8250 | 373 | 6.65 | 8.0 | L |
| pyrite seed 2 | 8250 | 376 | 6.65 | 6.0 | L |
| pyrite | 8250 | 348 | 4.88 | 3.0 | L |
| pyrite seed 2 | 8250 | 347 | 4.88 | 2.9 | L |
| pyrite | 8500 | 385 | 4.74 | 3.0 | L |
| pyrite | 8500 | 422 | 4.61 | 2.6 | L |
| pyrite | 8500 | 463 | 4.47 | 4.6 | L |

FIG. S1. Left figure shows the integrand of Eq. 1 (main text) from an ideal gas to liquid $SiO_2$ as function of $\lambda$ (i.e. from an ideal gas to liquid $SiO_2$) and the right figure shows the corresponding figure after changes of variables (i.e. the integrand in Eq. 1 as function $x$ for k = 0.8).

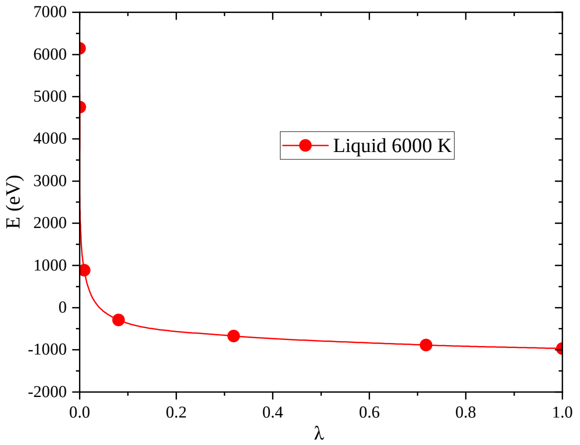


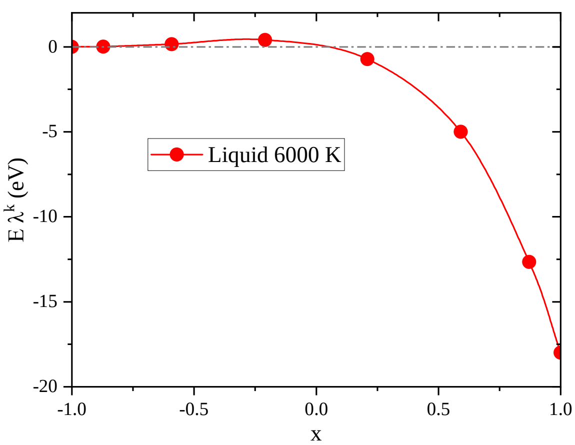


TABLE S2. Comparison of the integration steps (Eq. 1) for different values of $\lambda$ for the liquid at 6000 K and V = 1338.7189 $\AA^3$ with k = 0.8.

| **8 $\lambda$ Points** | | | | |
|---|---|---|---|---|
| x | $\omega$ | $\lambda$ | F($\lambda$) | $\delta$ F=F($\lambda$)$\times\omega\times\lambda^k$ |
| -1 | 0.035714286 | 0 | | 0 |
| -0.87174015 | 0.210704227 | 1.08469E-06 | 5821.04406 | 0.051862933 |
| -0.5917 | 0.341122692 | 0.000354607 | 4254.58257 | 6.302387661 |
| -0.209299 | 0.412458795 | 0.00965854 | 710.29847 | 17.89330751 |
| 0.209299 | 0.412458795 | 0.080819934 | -384.9497 | -53.05659254 |
| 0.5917 | 0.341122692 | 0.319268523 | -730.58131 | -249.9447735 |
| 0.87174 | 0.210704227 | 0.717922607 | -937.58839 | -378.8677001 |
| 1 | 0.035714286 | 1 | -1011.922 | -90.35017857 |
| | | | SUM | -747.9716865 |

| **10 $\lambda$ Points** | | | | |
|---|---|---|---|---|
| x | $\omega$ | $\lambda$ | F($\lambda$) | $\delta$ F=F($\lambda$)$\times\omega\times\lambda^k$ |
| -1 | 0.022222222 | 0 | | 0 |
| -0.91953391 | 0.133305991 | 1.05418E-07 | 6034.15304 | 0.005269114 |
| -0.73877387 | 0.224889342 | 3.80131E-05 | 6062.77289 | 0.992034249 |
| -0.47792495 | 0.292042684 | 0.001212034 | 2944.72489 | 9.982580909 |
| -0.16527896 | 0.327539761 | 0.012663589 | 498.47024 | 12.38479239 |
| 0.16527896 | 0.327539761 | 0.067142815 | -323.33949 | -30.5114202 |
| 0.47792495 | 0.292042684 | 0.220349427 | -643.94727 | -140.1929539 |
| 0.73877387 | 0.224889342 | 0.496667277 | -840.9888 | -270.1167602 |
| 0.91953391 | 0.133305991 | 0.814383498 | -969.52515 | -274.1649467 |
| 1 | 0.022222222 | 1 | -1011.922 | -56.21788889 |
| | | | SUM | -747.8392932 |

FIG. S2. Convergence of the total free energy as a function of the number of lambda points.

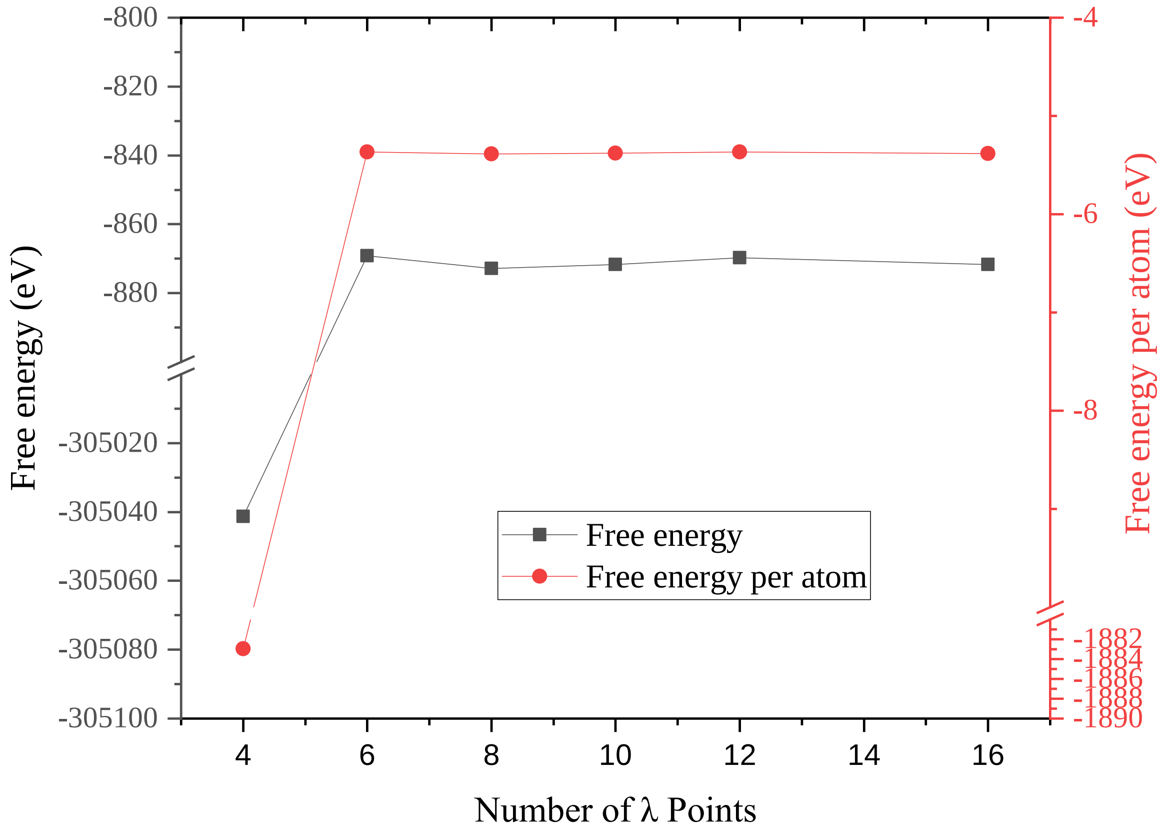

FIG. S3. Gibbs free energies for solid and liquid states calculated using TI. The melting points are calculated from linear fit to solid and liquid points. The solid and liquid simulation boxes have the same number of atoms. The solid phases are Stishovite, $\beta$-Stishovite and Pyrite optimized under different pressures respectively.

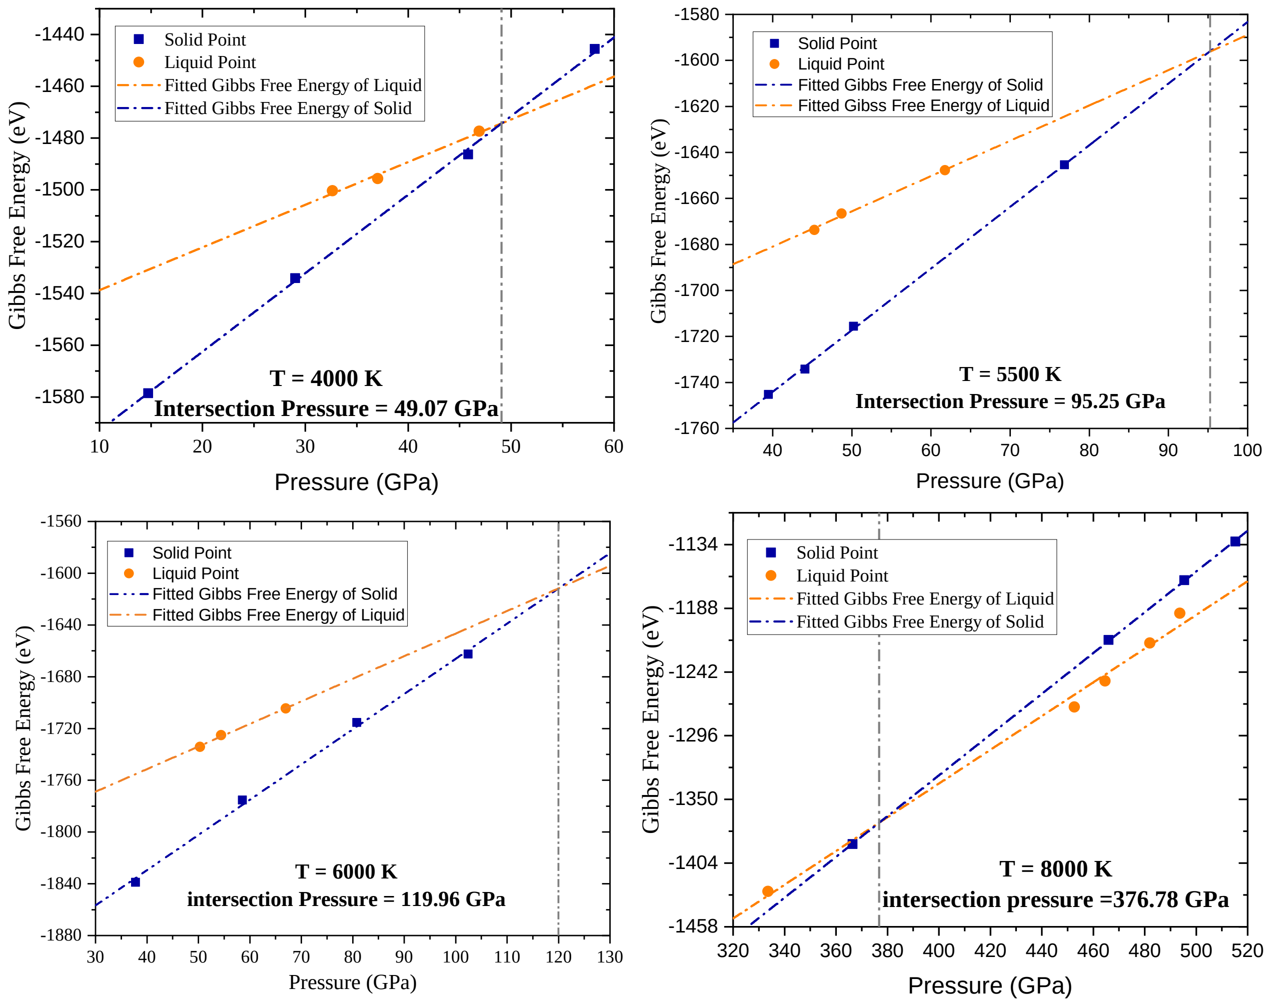

FIG. S4. Temperature and pressure evolutions of two typical Z Method MD runs. The thin lines show dumps every time-step whereas the thick lines are averaged properties over the previous 100 time-steps. Both trajectories start from the same initial crystal structure but with different initial temperatures. To calculate the waiting time for the system to melt we picked the time corresponding to the mid-point between the solid and liquid temperatures. Both show a clear temperature drop during melting. However, they show very different waiting times and liquid equilibrium temperatures which are used for determining melting temperature.

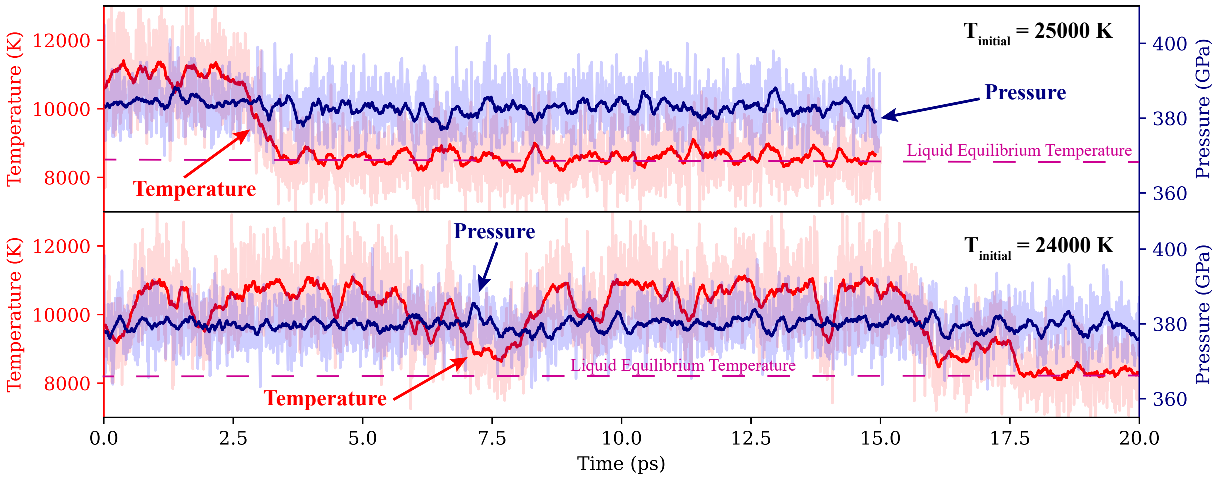

FIG. S5. Waiting Time analysis used in the Z method to calculate the melting temperatures at infinitive waiting time. The starting structure in the MD runs is Pyrite.

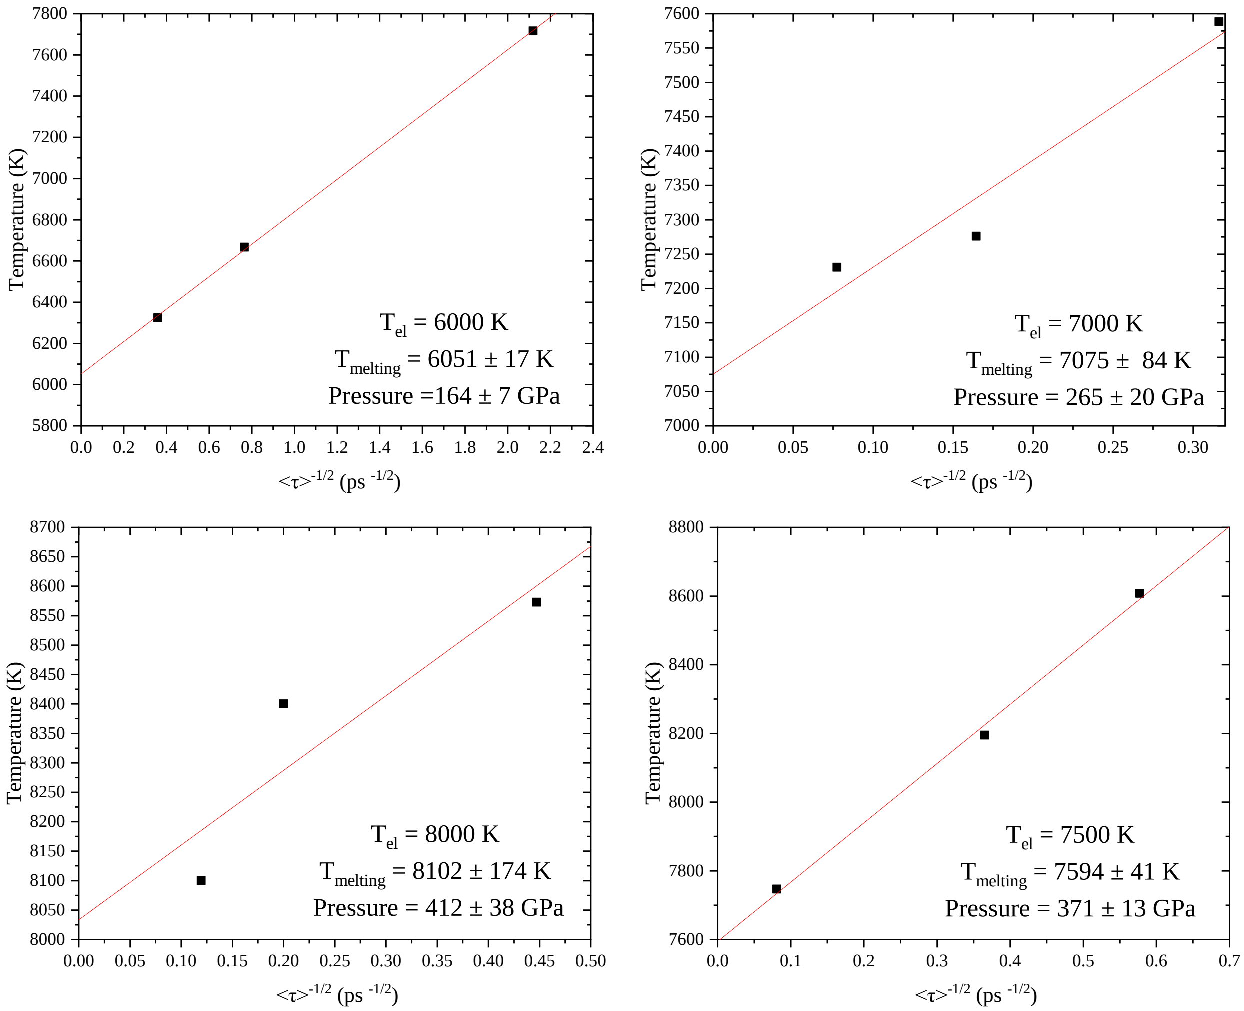

FIG. S6. Solid and liquid branches in MD-NVE runs for $SiO_2$ with $T_{\mathrm{el}}$ = 6000 K and 8000 K. The homogeneous melting temperatures are calculated from an intersection of a linear extrapolation of the solid branch runs and a vertical line drawn from the equilibrium melting point. The resulting $T_{\mathrm{h}}$ may therefore represent an upper bound to the "true" homogeneous melting temperature since the slope of the solid branch generally flattens near $T_{\mathrm{h}}$.

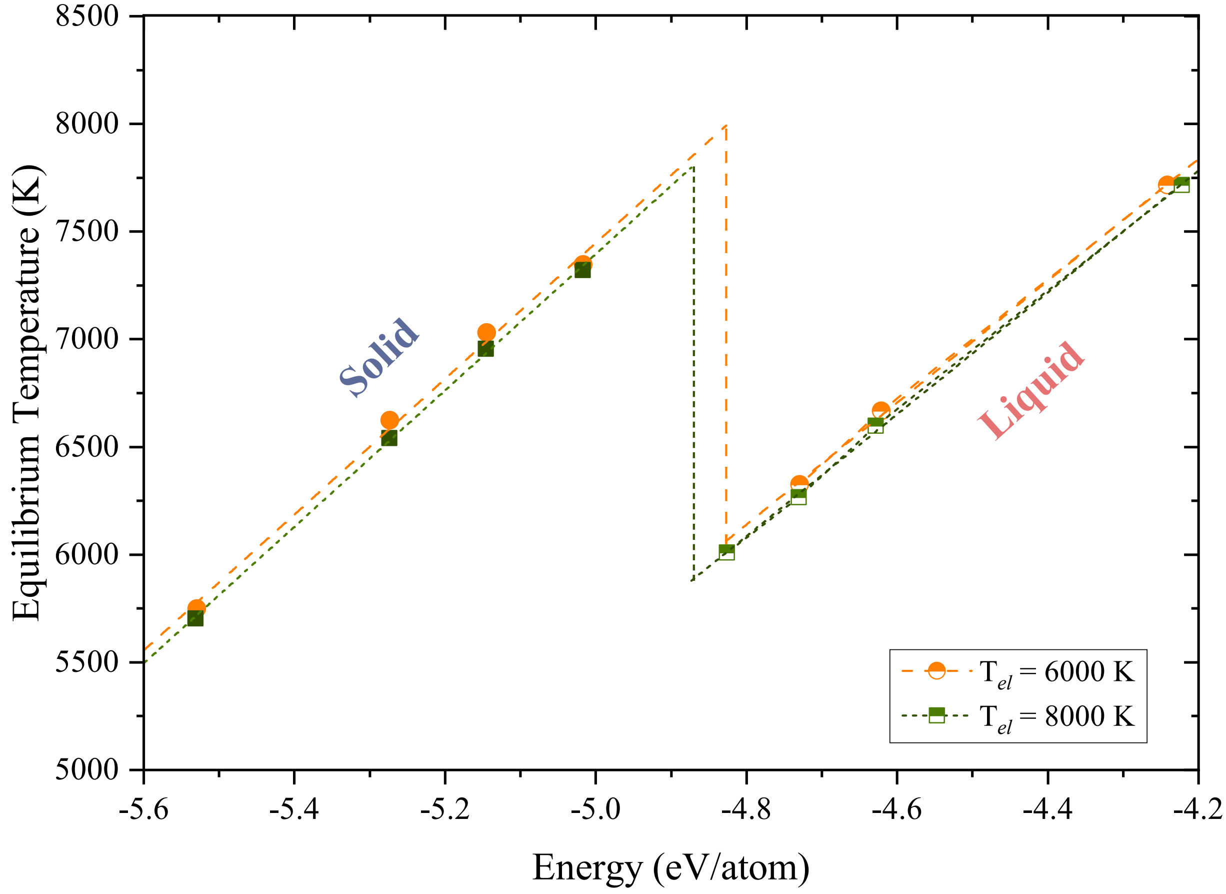

FIG. S7. Simulated XRD of silica melt at two temperatures and pressures along the melting curve. The main peak shifted towards the larger diffraction angle with the increase of pressure. The wavelength of the X-ray is set to 1.54059 Å

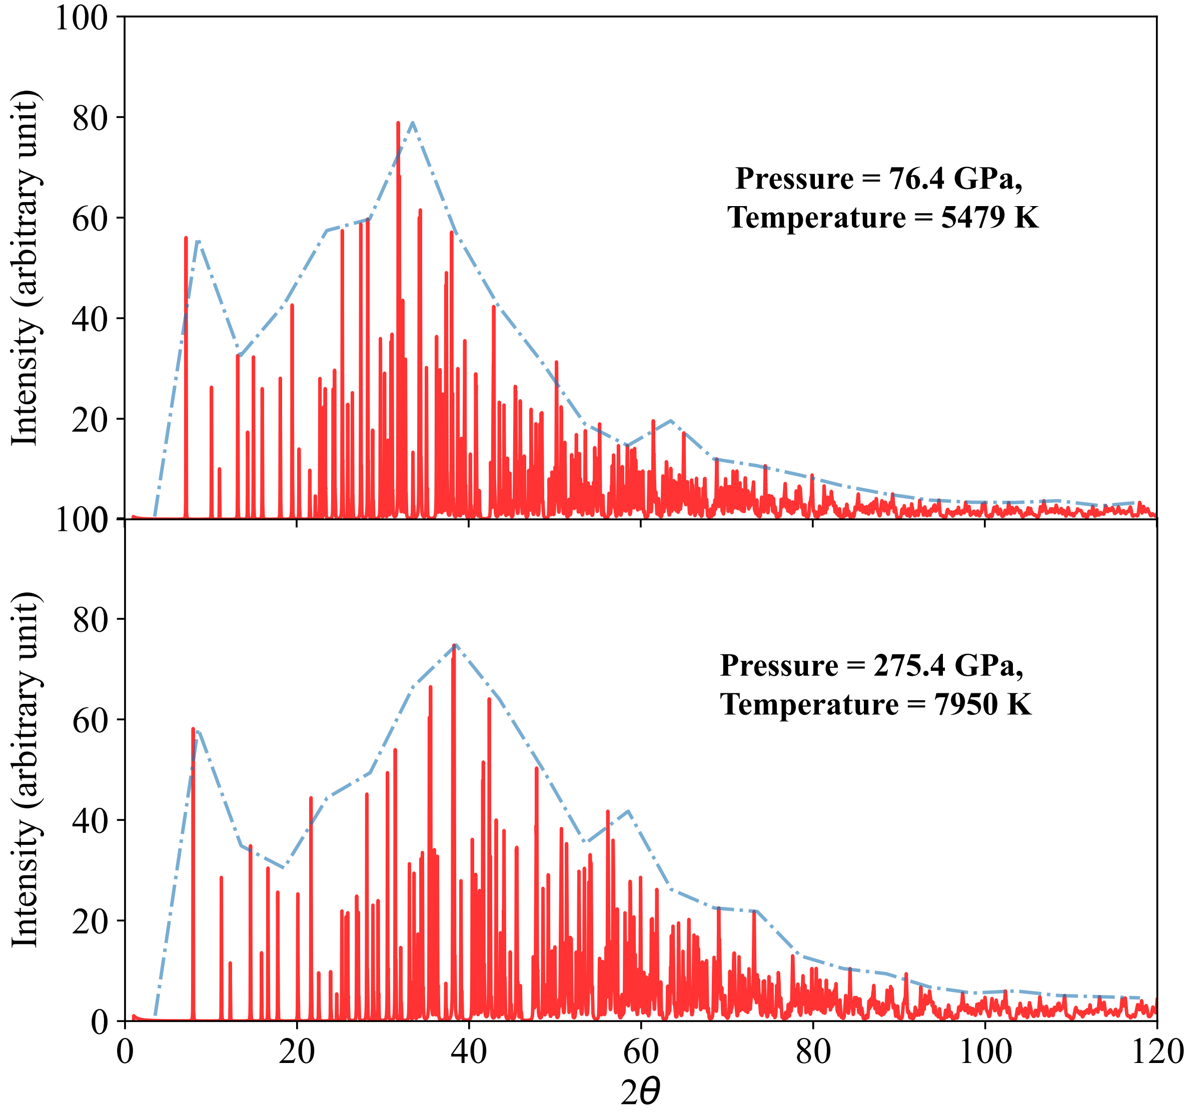

Supplement: Supplementary file 1 [file SupplementalInfo.pdf]
